# Supplementary material for: Programming evolution of geometry in shape-morphing sheets via spatiotemporal activation
Source: arXiv:2405.21024 ancillary file (2024-10-15)
Supplement: Supplementary file 1 [file SM.pdf]

# Supplementary Material for 'Programming evolution of geometry in shape-morphing sheets via spatiotemporal activation'

**Subject Areas:**
mechanics, geometry, applied mathematics

**Keywords:**
active materials, metric mechanics, shape-programmable systems

**Author for correspondence:**
Cyrus Mostajeran
e-mail: cyrussam.mostajeran@ntu.edu.sg

Daniel Duffy[1, 2], Itay Griniasty[3], John Biggins[1] and Cyrus Mostajeran[2]

[1]Department of Engineering, University of Cambridge,Cambridge CB2 1PZ, UK
[2]School of Physical and Mathematical Sciences, Nanyang Technological University, Singapore 637371, Singapore
[3]Laboratory of Atomic and Solid State Physics, Cornell University, Ithaca, New York 14853-2501, USA

# S1. Inverse design of material director

## (a) Director design for a target surface of revolution

Let $z = z(\rho)$ be a target surface of revolution expressed in cylindrical polar coordinates $(\rho, \phi, z)$. We seek to programme its metric in the in polar coordinates $(r, \theta)$ using a circularly symmetric director field characterized by a nematic alignment angle $\alpha = \alpha(r)$ such that $\hat{\boldsymbol{n}} = (\cos(\theta + \alpha), \sin(\theta + \alpha))$. As shown in [1], the components of the metric in $(r, \theta)$ coordinates take the form

$$\begin{cases} \bar{a}_{rr} & = \lambda^2 + \left(\lambda^{-2\nu} - \lambda^2\right)\sin^2(\alpha), \\ \bar{a}_{r\theta} & = \bar{a}_{\theta r} = -\frac{1}{2} r \left(\lambda^{-2\nu} - \lambda^2\right)\sin(2\alpha), \\ \bar{a}_{\theta\theta} & = r^2\left[\lambda^{-2\nu} - \left(\lambda^{-2\nu} - \lambda^2\right)\sin^2(\alpha)\right], \end{cases} \tag{S1}$$

where $\mathrm{d}l_A^2 = \bar{a}_{rr}\mathrm{d}r^2 + 2\bar{a}_{r\theta}\mathrm{d}r\mathrm{d}\theta + \bar{a}_{\theta\theta}\mathrm{d}\theta^2$. Since we impose circular symmetry, $\rho = \rho(r)$. The surface of revolution is characterized by two functions of $r$ that measure lengths across the surface: (i) $l_r(r)$, which measures the length from the smallest possible value of $r = r_0$, (usually $r_0 = 0$) up to $r$, and (ii) $l_\theta(r)$, which measures the circumference of the circle centred on the axis of symmetry of the surface corresponding to the coordinate $r$.

The length $l_\theta$ can be written as either $l_\theta(r) = 2\pi\rho(r)$ or $l_\theta(r) = 2\pi\sqrt{\bar{a}_{\theta\theta}(r)}$, which together imply

$$\rho(r) = \sqrt{\bar{a}_{\theta\theta}(r)}\,, \tag{S2}$$

while

$$l_r(r) = \int_0^{\rho(r)} \sqrt{1 + z'(\rho)^2}\mathrm{d}\rho, \tag{S3}$$

where $z'(\rho) = (\mathrm{d}z(\rho)/\mathrm{d}\rho)$. To express $l_r(r)$ in terms of the programmable metric, we first note that two curves $\Gamma_1$ and $\Gamma_2$ with polar parametric representations $(r, \theta) = (r_1(t), \theta_1(t))$ and $(r, \theta) = (r_2(t), \theta_2(t))$ are orthogonal with respect to the metric $\mathrm{d}l_A^2 = \bar{a}_{rr}\mathrm{d}r^2 + 2\bar{a}_{r\theta}\mathrm{d}r\,\mathrm{d}\theta + \bar{a}_{\theta\theta}\mathrm{d}\theta^2$, if and only if $\bar{a}_{rr}r_1'r_2' + \bar{a}_{r\theta}r_1'\theta_2' + \bar{a}_{\theta r}\theta_1'r_2' + \bar{a}_{\theta\theta}\theta_1'\theta_2' = 0$. The concentric circles on the undeformed sheet can be parametrised such that $r_1' = 0$ and $\theta_1' = 1$. Thus, the curve $(r(t), \theta(t))$ on the undeformed sheet whose image becomes orthogonal to the images of the concentric circles upon stimulation—the so-called 'proto-radial curve'—satisfies $\bar{a}_{\theta r}r' + \bar{a}_{\theta\theta}\theta' = 0$. That is, $\mathrm{d}\theta/\mathrm{d}r = -\bar{a}_{\theta r}/\bar{a}_{\theta\theta}$. The length of such a curve emanating from the origin is given by

$$l_r(r) = \int_0^r \sqrt{\bar{a}_{rr} + 2\left(\frac{\mathrm{d}\theta}{\mathrm{d}r}\right)\bar{a}_{r\theta} + \left(\frac{\mathrm{d}\theta}{\mathrm{d}r}\right)^2 \bar{a}_{\theta\theta}}\,\mathrm{d}r \tag{S4}$$

upon activation. Since $\mathrm{d}\theta/\mathrm{d}r = -\bar{a}_{\theta r}/\bar{a}_{\theta\theta}$, (S4) reduces to

$$l_r(r) = \int_0^r \frac{\sqrt{\bar{a}_{rr}\bar{a}_{\theta\theta} - \bar{a}_{r\theta}^2}}{\sqrt{\bar{a}_{\theta\theta}}}\mathrm{d}r = \lambda^{1-\nu}\int_0^r \frac{r\,\mathrm{d}r}{\sqrt{\bar{a}_{\theta\theta}}}, \tag{S5}$$

which combines with (S3) to give

$$\lambda^{1-\nu}\int_0^r \frac{r\,\mathrm{d}r}{\sqrt{\bar{a}_{\theta\theta}}} = \int_0^r \sqrt{1 + z'(\rho)^2}\frac{\mathrm{d}\rho}{\mathrm{d}r}\mathrm{d}r.$$

Upon differentiating with respect to $r$ and using (S2), we obtain

$$\lambda^{1-\nu}\frac{r}{\sqrt{\bar{a}_{\theta\theta}}} = \sqrt{1 + \left(z'(\sqrt{\bar{a}_{\theta\theta}})\right)^2}\frac{\mathrm{d}}{\mathrm{d}r}\sqrt{\bar{a}_{\theta\theta}} \tag{S6}$$

$$\Rightarrow \quad \lambda^{1-\nu}r = \frac{1}{2}\sqrt{1 + \left(z'(\sqrt{\bar{a}_{\theta\theta}})\right)^2}\frac{\mathrm{d}}{\mathrm{d}r}\bar{a}_{\theta\theta}. \tag{S7}$$

Integration with respect to $r$ now yields

$$\lambda^{1-\nu}(r^2 - r_0^2) = \int_{r_0}^{r} 2\lambda^{1-\nu} r \, \mathrm{d}r = \int_{\bar{a}_{\theta\theta}(r_0)}^{\bar{a}_{\theta\theta}(r)} \sqrt{1 + \left(z'(\sqrt{\bar{a}_{\theta\theta}})\right)^2} \, \mathrm{d}\bar{a}_{\theta\theta}, \tag{S8}$$

where we take $r_0 = 0$ and $\bar{a}_{\theta\theta}(r_0) = 0$ for a surface that intersects the axis of revolution.

## (b) Alternative director design for a paraboloid

Here we use the method of [2] to find a smooth director field solution to the paraboloid inverse design problem. To use the system of equations, we need the expression for the Gaussian curvature of the paraboloid given by $z = \frac{1}{2} a \rho^2$. The Gaussian curvature of the paraboloid is given by

$$K(\rho) = \frac{a^2}{(1 + a^2 \rho^2)^2}. \tag{S9}$$

Using the system of equations and numerical methods utilized in [2], we obtain a smooth director field for any specified choice of $a$ and $\Lambda$ given appropriate initial conditions on the director field (e.g. a director field line and the 'orthogonal dual' to it). An example with $a = 1.1$ and $\Lambda = 0.5$, $\nu = 1/2$ is illustrated in figure S1.

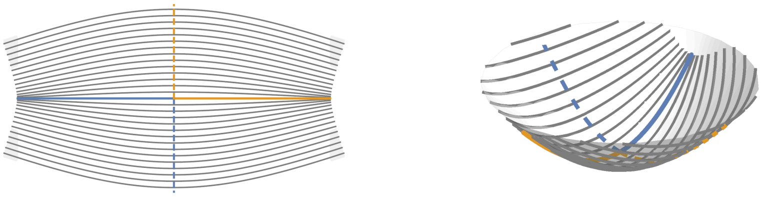

**Figure S1.** A smooth director field and its actuation to a target paraboloid of revolution $z = \frac{1}{2} a \rho^2$ with $a = 1.1$ for a target $\Lambda = 0.5$.

## (c) Director design on an initially curved surface

Consider two surfaces of revolution $\Sigma_i$ and $\Sigma_f$, given by $z_i = z_i(\rho_i)$ and $z_f = z_f(\rho_f)$, respectively. We seek to programme the surface of $\Sigma_i$ with a circularly symmetric director field that upon actuation results in a transition to $\Sigma_f$. Let $(r, \theta)$ denote geodesic polar coordinates on $\Sigma_i$ and $\hat{\boldsymbol{e}}_r$ and $\hat{\boldsymbol{e}}_\theta$ be unit vectors on $\Sigma_i$ in the radial and azimuthal directions. For simplicity, we assume that $r = 0$ when $\rho_i = 0$ so that the surfaces intersect the axis of revolution as in the case of paraboloids. We denote the director on $\Sigma_i$ by $\hat{\boldsymbol{n}}$ and take $\hat{\boldsymbol{n}}^\perp$ to be the orthogonal unit vector on $\Sigma_i$ such that

$$\hat{\boldsymbol{e}}_r = \cos\alpha(r)\hat{\boldsymbol{n}} + \sin\alpha(r)\hat{\boldsymbol{n}}^\perp, \quad \hat{\boldsymbol{e}}_{\theta\theta} = \sin\alpha(r)\hat{\boldsymbol{n}} - \cos\alpha(r)\hat{\boldsymbol{n}}^\perp, \tag{S10}$$

where $\alpha = \alpha(r)$ is the angle the director makes with the geodesic radial direction on $\Sigma_i$. The geodesic radius $r$ is related to $\rho_i$ by

$$r(\rho_i) = \int_0^{\rho_i} \sqrt{1 + (z_i'(\rho))^2} \, \mathrm{d}\rho. \tag{S11}$$

An infinitesimal variation $\mathrm{d}\boldsymbol{r}$ at $(r, \theta)$ on the surface $\Sigma_i$ takes the form

$$\mathrm{d}\boldsymbol{r} = \mathrm{d}r \, \hat{\boldsymbol{e}}_r + \rho_i(r)\mathrm{d}\theta \, \hat{\boldsymbol{e}}_{\theta\theta} \tag{S12}$$

$$= (\mathrm{d}r \cos\alpha + \rho_i(r) \sin\alpha \, \mathrm{d}\theta)\hat{\boldsymbol{n}} + (\mathrm{d}r \sin\alpha - \rho_i(r) \cos\alpha \, \mathrm{d}\theta)\hat{\boldsymbol{n}}^\perp, \tag{S13}$$

where $\rho_i = \rho_i(r)$ is the inverse of the function $r = r(\rho_i)$ given in (S11). Upon activation, the squared arclength $\mathrm{d}l^2 = |\mathrm{d}\boldsymbol{r}|^2$ becomes

$$\mathrm{d}l_A^2 = \left|\lambda(\mathrm{d}r\cos\alpha + \rho_i(r)\sin\alpha\,\mathrm{d}\theta)\hat{\boldsymbol{n}} + \lambda^{-\nu}(\mathrm{d}r\sin\alpha - \rho_i(r)\cos\alpha\,\mathrm{d}\theta)\hat{\boldsymbol{n}}^{\perp}\right|^2 \tag{S14}$$

$$= (\lambda^2c^2 + \lambda^{-2\nu}s^2)\,\mathrm{d}r^2 + 2(\lambda^2 - \lambda^{-2\nu})\rho_i(r)cs\,\mathrm{d}r\mathrm{d}\theta + \rho_i(r)^2(\lambda^2s^2 + \lambda^{-2\nu}c^2)\,\mathrm{d}\theta^2, \tag{S15}$$

where $s = \sin\alpha$ and $c = \cos\alpha$. This yields metric components

$$\begin{cases} \bar{a}_{rr} &= \lambda^2 + \left(\lambda^{-2\nu} - \lambda^2\right)\sin^2(\alpha), \\ \bar{a}_{r\theta} &= \bar{a}_{\theta r} = -\frac{1}{2}\rho_i(r)\left(\lambda^{-2\nu} - \lambda^2\right)\sin(2\alpha), \\ \bar{a}_{\theta\theta} &= \rho_i(r)^2\left[\lambda^{-2\nu} - \left(\lambda^{-2\nu} - \lambda^2\right)\sin^2(\alpha)\right], \end{cases} \tag{S16}$$

on the actuated surface. Repeating the analysis in subsection S1(a) with this metric, we find that the director field $\alpha = \alpha(r)$ for the inverse design problem is determined by

$$\int_0^r 2\lambda^{1-\nu}\rho_i(r)\mathrm{d}r = \int_0^{\bar{a}_{\theta\theta}(r)} \sqrt{1 + \left(z_f'(\sqrt{\bar{a}_{\theta\theta}})\right)^2}\,\mathrm{d}\bar{a}_{\theta\theta}$$

$$\Rightarrow \quad \int_0^{\rho_i} 2\lambda^{1-\nu}\rho\sqrt{1 + (z_i'(\rho))^2}\,\mathrm{d}\rho = \int_0^{\bar{a}_{\theta\theta}(r)} \sqrt{1 + \left(z_f'(\sqrt{\bar{a}_{\theta\theta}})\right)^2}\,\mathrm{d}\bar{a}_{\theta\theta}, \tag{S17}$$

## S2. Inverse-problem PDEs

Our $\lambda$-inverse problem can be formulated as follows: We are given $\hat{\boldsymbol{n}} = (\cos(\psi(x,y)), \sin(\psi(x,y)))$ on the $x-y$ plane, and we denote by $\boldsymbol{R}_\psi(x,y)$ the standard $2\times2$ matrix that rotates vectors anticlockwise by $\psi$. Given also a curved target surface inscribed with coordinates $(X^1, X^2)$, we consider flattened surfaces lying in the $x-y$ plane, described by mappings $x(X^1, X^2)$, $y(X^1, X^2)$. The corresponding deformation gradient

$$\boldsymbol{F} \equiv \begin{pmatrix} \partial x/\partial X^1 & \partial x/\partial X^2 \\ \partial y/\partial X^1 & \partial y/\partial X^2 \end{pmatrix}. \tag{S1}$$

A solution of the inverse problem must have the following property: upon activation each infinitesimal element of the sample in the $x-y$ plane is mapped to the target by some continuous deformation with a particular form at each point, namely stretches/compressions by factors $\lambda$ along $\hat{\boldsymbol{n}}$ and $\lambda^{-\nu}$ orthogonally, followed by some position-dependent 3D rigid-body motion. This condition is equivalent to the following restriction on the reverse (target→planar) mapping: for every infinitesimal element of the target, the mapping first rigidly rotates and translates that element into the $x-y$ plane in some way, then merely stretches/compresses by factors $1/\lambda$ along $\hat{\boldsymbol{n}}$ and $\lambda^\nu$ orthogonally. At any particular chosen point on the target, we can use suitable locally Cartesian coordinates $(X^1, X^2) = (X, Y)$ to write this restriction as

$$\boldsymbol{F} \equiv \begin{pmatrix} \partial_X x & \partial_Y x \\ \partial_X y & \partial_Y y \end{pmatrix} = \boldsymbol{R}_\psi \begin{pmatrix} 1/\lambda & 0 \\ 0 & \lambda^\nu \end{pmatrix} \boldsymbol{R}_\psi^{\mathrm{T}}\boldsymbol{Q}$$

$$= \begin{pmatrix} \cos\psi & -\sin\psi \\ \sin\psi & \cos\psi \end{pmatrix} \begin{pmatrix} 1/\lambda & 0 \\ 0 & \lambda^\nu \end{pmatrix} \begin{pmatrix} \cos\omega & -\sin\omega \\ \sin\omega & \cos\omega \end{pmatrix}, \tag{S2}$$

where in the final equality we have absorbed $\boldsymbol{R}_\psi^{\mathrm{T}}$ into the general rotation $\boldsymbol{Q}$ to yield a new general rotation that we parameterise with $\omega$. (We do not need to include a possible reflection in $\boldsymbol{Q}$, as long as the coordinates $(X^1, X^2)$ are chosen to have the appropriate 'orientation' locally.)

The energy density $W_s$ of the main text penalises deviations of $\boldsymbol{F}$ from the form (S2), underpinning our numerical approach to finding solutions, but the condition (S2) in fact directly defines (component-wise) four equations for four unknowns: $x$, $y$, $\lambda$ and $\omega$. To simplify our analysis going forward, we utilize a natural coordinate system for the $x-y$ plane, based on the director field $\hat{\boldsymbol{n}}$, following ref. [3]. These coordinates $(u, v)$ exist for any sufficiently smooth $\hat{\boldsymbol{n}}$,

and have the property that $v$ is constant along integral curves of $\hat{\boldsymbol{n}}$ while $u$ is constant along integral curves of $\hat{\boldsymbol{n}}_\perp$, where $\hat{\boldsymbol{n}}_\perp$ is everywhere orthogonal to $\hat{\boldsymbol{n}}$. Thus the basis vectors for the $u - v$ system are proportional to $\hat{\boldsymbol{n}}$ and $\hat{\boldsymbol{n}}_\perp$, yielding

$$\begin{pmatrix} \partial x/\partial u & \partial x/\partial v \\ \partial y/\partial u & \partial y/\partial v \end{pmatrix} = \begin{pmatrix} \alpha\cos\psi & -\beta\sin\psi \\ \alpha\sin\psi & \beta\cos\psi \end{pmatrix} = \begin{pmatrix} \cos\psi & -\sin\psi \\ \sin\psi & \cos\psi \end{pmatrix} \begin{pmatrix} \alpha & 0 \\ 0 & \beta \end{pmatrix} \tag{S3}$$

where $\alpha$ and $\beta$ are some functions of position $(u, v)$. (We use the symbols $\alpha$ and $\beta$ for consistency with ref. [3]; this usage is unrelated to that in other sections and in the main text.) Splitting the first matrix in (S2) into two via chain rule, then substituting (S3), we can cancel $\boldsymbol{R}_\psi$ to find

$$\begin{pmatrix} \partial_X u & \partial_Y u \\ \partial_X v & \partial_Y v \end{pmatrix} = \begin{pmatrix} 1/(\alpha\lambda) & 0 \\ 0 & \lambda^\nu/\beta \end{pmatrix} \begin{pmatrix} \cos\omega & -\sin\omega \\ \sin\omega & \cos\omega \end{pmatrix}. \tag{S4}$$

This system quickly yields

$$\lambda = \left( |\alpha| \sqrt{(\partial_X u)^2 + (\partial_Y u)^2} \right)^{-1},$$

$$\sin\omega = \beta\lambda^{-\nu}\partial_X v, \tag{S5}$$

$$\cos\omega = \beta\lambda^{-\nu}\partial_Y v, \tag{S6}$$

allowing us to eliminate $\lambda$ and $\omega$ in (S4). Doing so leaves two equations, which we write compactly as

$$\nabla_i u = \gamma(u, v)|\nabla u|^{1+\nu}\varepsilon_{ij}\nabla^j v \tag{S7}$$

where $i$ runs over coordinates and we have defined $\gamma \equiv \beta\alpha^{-1}|\alpha|^{1+\nu}$, which is fully determined by the director pattern. Now, we derived (S7) as a condition at a single arbitrary point on the target, using coordinates $(X, Y)$ that are locally Cartesian at that point. In those coordinates $\varepsilon_{ij}$ is the standard Levi-Civita symbol, but if we take $\varepsilon_{ij}$ to denote more generally the components of the Levi-Civita *tensor* ( [4] Sec. 2.8), then (S7) is manifestly fully tensorial ('covariant') with respect to the coordinate system inscribing the target surface, and therefore holds in *any* coordinates $(X^1, X^2)$. Thus the inverse problem is reduced to that of solving (S7) as a fully nonlinear first-order system of PDEs on the target surface.

Note that (S7) immediately implies the elegant relation $\nabla u \cdot \nabla v = 0$. Note also that in the case $\nu = -1$, the director pattern must become irrelevant to our inverse problem, so WLOG we may set $\psi = 0$, $u = x$, $v = y$, and hence $\alpha = \beta = \gamma = 1$. Then (S7) reduces to exactly the (covariant) Cauchy-Riemann equations, as it should, since the $\nu = -1$ inverse problem is exactly that of conformal flattening [5].

Let us now classify the nonlinear PDE system (S7), essentially following ref. [6] (Chap. 3 Sec. 2 and Chap. 5 Sec. 1.7). On both sides of (S7), we multiply by $|\nabla u|^{-1-\nu}$ then take the partial derivative with respect to the coordinate $X^2$, which yields a coupled pair of second-order quasilinear PDEs. Then for convenience we choose to use locally Cartesian coordinates $(X, Y) = (X^1, X^2)$ to examine the quasilinear PDEs at a point on the target; thus the metric components' values are given by $\mathrm{diag}(1, 1)$ while their first derivatives vanish. By defining $p \equiv \partial_X u$, $q \equiv \partial_Y u$, $j \equiv \partial_X v$, and $k \equiv \partial_Y v$, the two second-order equations at the examination point become first order. Supplementing with the four equations $q = \partial_Y u$, $k = \partial_Y v$, $\partial_Y p = \partial_X q$, $\partial_Y j = \partial_X k$ yields a quasilinear first-order six-equation system that can be written

$$\boldsymbol{A}\partial_X \boldsymbol{h} + \boldsymbol{B}\partial_Y \boldsymbol{h} + \boldsymbol{c} = 0, \tag{S8}$$

where $\boldsymbol{h} = (u, v, p, q, j, k)$. The matrices $\boldsymbol{A}$ and $\boldsymbol{B}$ and the vector $\boldsymbol{c}$ all depend on $\boldsymbol{h}$, and are somewhat cumbersome. We then calculate the roots of the characteristic determinant equation

$\det(\boldsymbol{A} - \sigma \boldsymbol{B}) = 0$, which are $\sigma = 0$ (repeated $4\times$) and

$$\sigma = \frac{(1+\nu)pq \pm \sqrt{\nu\left(p^2+q^2\right)^2}}{\nu q^2 - p^2}. \tag{S9}$$

Observe that the latter pair of roots are real for $\nu > 0$ and complex for $\nu < 0$. A system such as (S8) is classed as hyperbolic if it has real roots, and elliptic if it does not. The $\sigma = 0$ roots are always real, but are a mere artefact of the differentiation we used to obtain a quasilinear system; they are trivial and to be ignored as far as classification of (S7) is concerned. This is demonstrated by again considering $\nu = -1$: The $\sigma = 0$ roots remain in that case, but as discussed earlier (S7) reduce to the Cauchy-Riemann equations, which are *certainly* elliptic, because they are solved by harmonic functions satisfying the quintessentially elliptic Laplace equation [5]. Thus, based on the two non-trivial roots, we conclude that our inverse problem PDEs (S7) are hyperbolic for $\nu > 0$ and elliptic for $\nu < 0$.

## S3. Inverse-problem examples: extra figures

Supplementary data for our 'twister' and 'bending-channel' $\lambda$-inverse examples are presented in Figs S2, S3 and S4.

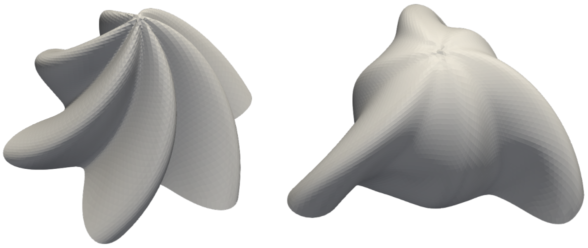

**Figure S2.** Left: A 'twister' surface with six lobes, as opposed to the three-lobe version presented in the main text and Fig. S3. Right: The bend-minimizing isometry (computed approximately using MorphoShell) is a decidedly different shape to that on the left, even exhibiting a different degree of axial symmetry (3-fold instead of 6-fold). This example illustrates that, in general, target surfaces must be chosen with some care when undertaking purely metric-based shape programming.

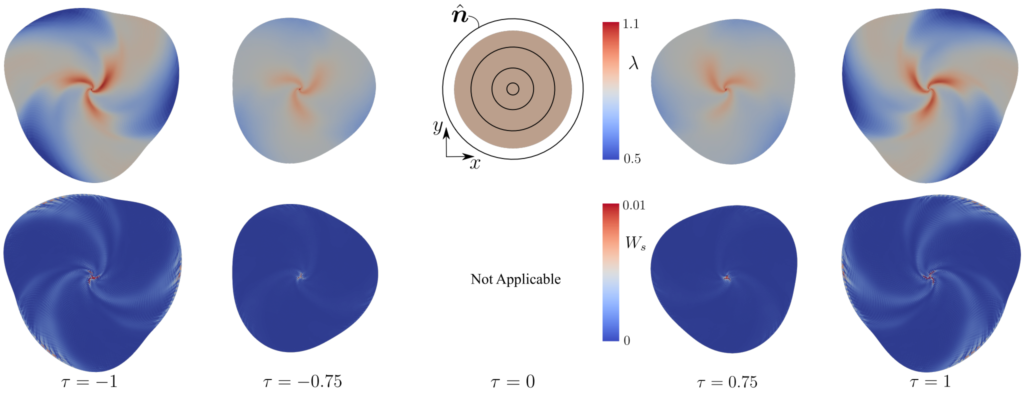


**Figure S3.** Row 1: Copy of row 4 of Fig. 6 in the main text. Solutions to the $\lambda$-inverse problem for a 'twister' family of target surfaces and an azimuthal director field. Row 2: The same solutions as in row 1, coloured by dimensionless energy $W_s$, whose smallness indicates the high quality of our numerical results. In each case $W_s < 0.01$ in at least 99.9% of the $\sim 18000$ mesh triangles.

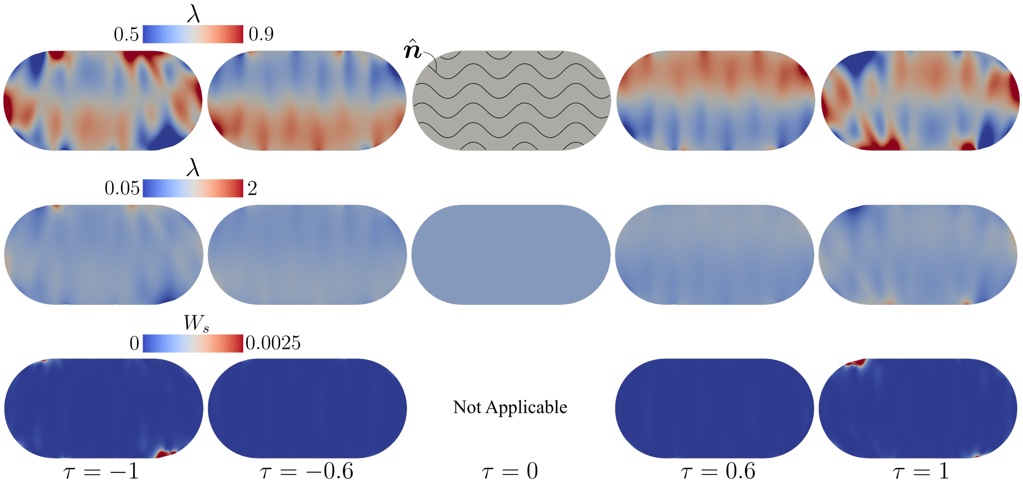


**Figure S4.** Row 1: Copy of row 4 of Fig. 7 in the main text. Solutions to the $\lambda$-inverse problem for a 'bending-channel' family of target surfaces and an oscillatory director field. Some of these colours clip/saturate the scale. Row 2: The same solutions as in row 1, but coloured using a different colour scale so that no clipping occurs. Row 3: The same solutions again, coloured by dimensionless energy $W_s$, whose smallness indicates the high quality of our numerical results. In each case $W_s < 0.001$ in at least 99.8% of mesh triangles. We attribute the localized patches of higher $W_s$ in the $|\tau| = 1$ solutions to the fact that $\lambda$ was very small in these regions, so the relevant mesh triangles became correspondingly large (in their dynamical deformed states), and thus locally the mesh did not 'resolve' the director pattern particularly well. (A simple adaptive re-meshing procedure could eliminate such effects.) Note, however, that $W_s$ remained fairly small even within these patches, only exceeding $0.01$ in $\sim 10$ of the mesh's $\sim 10^5$ triangles.

## References


1. Mostajeran C, Warner M, Ware TH, White TJ. 2016 Encoding Gaussian curvature in glassy and elastomeric liquid crystal solids. *Proceedings of the Royal Society A: Mathematical, Physical and Engineering Sciences* **472**, 20160112.
2. Griniasty I, Aharoni H, Efrati E. 2019 Curved Geometries from Planar Director Fields: Solving the Two-Dimensional Inverse Problem. *Physical review letters* **123**, 127801.
3. Niv I, Efrati E. 2018 Geometric frustration and compatibility conditions for two-dimensional director fields. *Soft matter* **14**, 424–431.
4. Carroll SM. 2019 *Spacetime and geometry*. Cambridge University Press.
5. Sawhney R, Crane K. 2017 Boundary First Flattening. *ACM Trans. Graph.* **37**. (10.1145/3132705)
6. Courant R, Hilbert D. 1962 *Methods of Mathematical Physics* vol. 2. Wiley-VCH.
